# Supplementary material for: CAMS: CAnonicalized Manipulation Spaces for Category-Level Functional Hand-Object Manipulation Synthesis
Source: arXiv:2303.15469 source file (2023-03-25)
Supplement: Supplementary file 1 [file supp.tex]

\section{Overview}

In the supplementary paper, we first present the details of our method (Section~\ref{sec:method_details}), our evaluation metrics (Section~\ref{sec:metric_details}), our experiments (Section~\ref{sec:experimental_details}), and the data processing (Section~\ref{sec:data_processing}), respectively. We then compare our approach with an additional baseline (Section~\ref{sec:additional_baseline}) and conduct more ablation studies (Section~\ref{sec:additional_ablation}) to verify the effectiveness of different modules in our method.
% We finally present more visualization in Section~\ref{sec:visualization} and our supplementary \textbf{video}.

Besides the paper, we strongly recommend watching our \textbf{video} to visualize our approach and its synthesis effects.

\section{Method Details}
\label{sec:method_details}

Section~\ref{subsec:loss_planner} shows the loss design of our \textbf{planner} (see Section 4.2 in the main paper) in detail, while Section~\ref{subsec:loss_synthesizer} provides the details of loss functions in our \textbf{synthesizer} (see Section 4.3 in the main paper).
In the following subsections, we use hatted symbols (\eg $\hat{\mathbf{C}}_{i,j}$) to denote network
predictions, and vise versa (\eg $\mathbf{C}_{i,j}$) for the ground truth values.

\subsection{Definitions of Loss Functions in Planner}
\label{subsec:loss_planner}

In this section, any notation with hat indicates a ground truth value. We first define our BCE loss $\mathcal{L}_{flag}$ as:

\begin{equation}
\begin{split}
\mathcal{L}_{flag} = & \sum_{i=1}^{5}\sum_{j=1}^M\sum_{k=1}^N BCE(\mathbf{\hat c}_{ijk}, \mathbf{c}_{ijk}) \\
& + \sum_{i=1}^{5}\sum_{j=1}^M\sum_{k=1}^N\sum_{t=1}^T BCE(\mathbf{\hat f}_{n,ijkt}, \mathbf{f}_{n,ijkt}) \\
& + \sum_{i=1}^{5}\sum_{j=1}^M\sum_{k=1}^N\sum_{t=1}^T BCE(\mathbf{\hat f}_{c,ijkt}, \mathbf{f}_{c,ijkt}),
\end{split}
\end{equation}

in which the subscript $1\le t\le T$ indicates a sampled frame index in time-continuous part.

Two $L_2$ loss functions $\mathcal{L}_{tip}$ and $\mathcal{L}_{vec}$ are defined as:

\begin{equation}
\begin{split}
\mathcal{L}_{tip} = 
& \sum_{i=1}^{5}\sum_{j=1}^M\sum_{k=1}^N\sum_{t=1}^T
\mathbf {\hat c}_{ijk}(\|\hat{\mathbf{J}}_{start,ijkt}^{tip}-\mathbf{J}_{start,ijkt}^{tip}\|_2^2 \\
& + \|\hat{\mathbf{J}}_{end,ijk}^{tip}-\mathbf{J}_{end,ijk}^{tip}\|_2^2), \\
\mathcal{L}_{vec}= & \sum_{joint \in \{dip,pip,mcp,root\}} \mathcal{L}_{vec}(joint), \\
\mathcal{L}_{vec}(joint)= & \sum_{i=1}^{5}\sum_{j=1}^M\sum_{k=1}^N\sum_{t=1}^T
\mathbf {\hat c}_{ijk}(\|\hat{\mathbf{D}}_{start,ijkt}^{joint}-\mathbf{D}_{start,ijkt}^{joint}\|_2^2 \\
& + \|\hat{\mathbf{D}}_{end,ijk}^{joint}-\mathbf{D}_{end,ijk}^{joint}\|_2^2),
\end{split}
\end{equation}
where $j$ denotes the index of the stage that contains frame $t$, and $k \in \{1,2,3,root\}$ indicates different joints on a finger.

The KL-Divergence loss $\mathcal{L}_{KLD}$ is defined as:

\begin{equation}
\mathcal{L}_{KLD}=KL(\mathbf{Q}(z|\mu, \theta^2) \| \mathcal{N}(0, I)).
\end{equation}

\subsection{Definitions of Loss Functions in Synthesizer}
\label{subsec:loss_synthesizer}

The L2 loss $\mathcal{L}_{tip}$ for measuring fingertip positions is defined as:

\begin{equation} \label{eq:fit_loss_tip}
\begin{split}
    \mathcal{L}_{\mathrm{tip}}(\theta_t) &=
    \sum_{i=1}^{5} \sum_{k=1}^{N} 
    (\mathbf{f}_n)_{i,t,k} \\
    & \lVert\mathrm{MANO}(\mathbf{J}^{tip}_{i};\beta,\theta_t)-\mathbf{J}^{tip}_{i,t,k}\rVert^2,
\end{split}
\end{equation}

where $\mathrm{MANO}(\mathbf{J}^{tip}_{i};\beta,\theta_t)$\cite{mano} computes the tip position of finger $i$ given the MANO parameter $\{\beta, \theta_t\}$, and $\mathbf{J}^{tip}_{i,t,k}$ indicates the target fingertip position in the $t$-th frame with respect to the information from the $k$-th object part, which is the linear interpolation from the two directly predicted fingertip positions $\{(\mathbf{J}_1)^{tip}_{i,t,k},(\mathbf{J}_2)^{tip}_{i,t,k}\}$ in the finger embeddings $(\mathbf{F}_1)_{i,t,k},(\mathbf{F}_2)_{i,t,k}$. The target fingertip position is then transformed into the world coordinate frame.

The L2 loss $\mathcal{L}_{joint}$ for measuring finger joint direction vectors is defined as:

\begin{equation} \label{eq:fit_loss_joint}
\begin{split}
    \mathcal{L}_{\mathrm{joint}}(\theta_t) = & \sum_{i=1}^{5}\sum_{k=1}^{N}\sum_{joint}(\mathbf{f}_n)_{i,t,k} \\
    & \lVert\mathrm{MANO}(\mathbf{J}^{joint}_{i};\beta,\theta_t) \\
    -& \mathrm{MANO}(\mathbf{J}^{tip}_{i};\beta,\theta_t)-\mathbf{D}^{joint}_{i,t,k}\rVert^2,
\end{split}
\end{equation}

where $\mathrm{MANO}(\mathbf{J}^{joint}_{i};\beta,\theta_t)$ is each of the joint positions of finger $i$ given the MANO parameter $\{\beta,\theta_t\}$, and $\mathbf{D}^{joint}_{i,t,k}$ is the target joint orientation, similarly interpolated and transformed from the predicted $\mathbf{D}$ as in Equation~\eqref{eq:fit_loss_tip}.

The temporal smoothness loss $\mathcal{L}_{\mathrm{smooth}}$ is defined as:

\begin{equation} \label{eq:fit_loss_smooth}
\begin{split}
    \mathcal{L}_{\mathrm{smooth}}(\theta) &= \sum_{t=2}^{T} \lVert\theta_{t}-\theta_{t-1}\rVert^2.
\end{split}
\end{equation}

We use $j(t)$ to denote the stage index containing the time $t$. To define the contact loss $\mathcal{L}_{\mathrm{contact}}$, we first find all frame-finger index tuples $(i,t,k)$ satisfying $(\mathbf{f}_c)_{i,t,k}=1$, indicating where contact should take place. For each of such tuple $(i,t,k)$, we search for a local surface section $(\mathbf{M}^\prime_{k})_{t,i}$ of the contacting object part $\mathbf{M}_k$. $(\mathbf{M}^\prime_{k})_{t,i}$ is set to be the closest section to the predicted reference frame $\mathbf{V}_{i,j(t),k}$ where all the vertex normals in such a local section are within a fixed included angle range $\alpha=45^\circ$ compared to the predicted contact normal $\mathbf{N}_{i,j(t),k}$. We calculate the signed distances $\{\mathbf{d}_{i,t,k,l}\}_{l=1}^{n(i)}$ from each of the finger vertices to $(\mathbf{M}^\prime_{k})_{t,i}$, as well as the corresponding nearest points $\{\mathbf{p}_{i,t,k,l}\}_{l=1}^{n(i)}$ on $(\mathbf{M}^\prime_{k})_{t,i}$, where $n(i)$ is the number of vertices on the $i$-th finger. The contact loss $\mathcal{L}_{\mathrm{contact}}$ is designed to attract the nearby finger vertices to the local surface section:

\begin{equation} \label{eq:syn_contact_loss}
\begin{split}
    \mathcal{L}_{\mathrm{contact}}(\theta^\prime) &= \sum_{(\mathbf{f}_c)_{i,t,k}=1}\sum_{l=1}^{n(i)} c_{i,t,k,l} \\
    &\cdot \lVert\mathrm{MANO}(\mathbf{vertex}_{i,l};\beta,\theta^\prime_t) - \mathbf{p}_{i,t,k,l}\rVert^2,
\end{split}
\end{equation}
where $c_{i,t,k,l}=e^{-(\lVert\mathbf{d}_{i,t,k,l}\rVert^2-\min_{l^*}\lVert\mathbf{d}_{i,t,k,l^*}\rVert^2)}$ provides centralized coefficients for such finger vertices.

Similar to $\{\mathbf{d}_{i,t,k,l}\}_{l=1}^{n(i)}$ and $\{\mathbf{p}_{i,t,k,l}\}_{l=1}^{n(i)}$, we compute $\{\mathbf{d}^\prime_{i,t,k,l}\}_{l=1}^{n(i)}$ and $\{\mathbf{p}^\prime_{i,t,k,l}\}_{l=1}^{n(i)}$ that are towards the whole object part $\mathbf{M}_k$ but not the local $(\mathbf{M}^\prime_{k})_{t,i}$, and thus define the penetration loss $\mathcal{L}_{\mathrm{penetr}}$ as:

\begin{equation} \label{eq:syn_penetr_loss}
\begin{split}
    \mathcal{L}_{\mathrm{penetr}}(\theta^\prime) &= \sum_{i,t,k}\sum_{l=1}^{n(i)} p_{i,t,k,l}\cdot c^\prime_{i,t,k,l} \\
    &\cdot \lVert\mathrm{MANO}(\mathbf{vertex}_{i,l};\beta,\theta^\prime_t) - \mathbf{p}^\prime_{i,t,k,l}\rVert^2,
\end{split}
\end{equation}

where $c^\prime_{i,t,k,l}=e^{-(\lVert\mathbf{d}^\prime_{i,t,k,l}\rVert^2-\min_{l^*}\lVert\mathbf{d}^\prime_{i,t,k,l^*}\rVert^2)}$, and $p_{i,t,k,l}=1$ only if the hand vertex penetrates the object part in frame $t$.

% \modify{how to present the following contents? @zjt}
% \textbf{In Appendix or Algorithm explain the detailed steps of generating contact reference and finger embedding}
% Given hand configuration from parametric hand model MANO \cite{mano} and object 6D pose in world frame that describe the manipulation over the course of intersection of $\mathbf{T}$ frames, we first transform the entire scene to canonical object frame and get corresponding hand joint vertices $\mathbf{J}=(\mathbf{J}^t)_{1\leq t \leq T}, \mathbf{J}^t\in \mathbb{R}^{M\times 3}$ and object vertices $\mathbf{O}=(\mathbf{O}^t)_{1\leq t \leq T}, \mathbf{O}^t\in \mathbb{R}^{N\times 3}$. Without loss of generality, we sample one frame where contact happens from the sequence and introduce how to represent the contact of $\mathbf{J}^t$ and $\mathbf{O}^t$ in canonicalized manipulation space. Here, we define a contact on object surface as $\mathbf{F}(\mathbf{J}^t, \mathbf{O}^t)=\{(\mathbf{V}_i, \mathbf{N}_i)\}_{i=1}^M$

\section{Metric Details}
\label{sec:metric_details}

In this section, we introduce our evaluation metrics (see Section 5.4 in the main paper) in detail.

\subsection{Contact-Movement Consistency}
\label{subsec:CM_Consist}

We evaluate whether the object's movement can align with the contact forces produced by hand-object contacts, using the same physics model as in ManipNet\cite{zhang2021manipnet}.

Following \cite{zhang2021manipnet}, for each part of the object in a single video frame, we calculate the change of linear momentum $\dot{P}$ and angular momentum $\dot{L}$.

\begin{equation}\label{eq:eval_dynamics}
\begin{split}
& P(t)=Mv(t), \\
& \dot{P}(t)=M\dot{v}(t), \\
& L(t)=I(t)\omega(t), \\
& \dot{L}(t)=\dot{I}(t)\omega(t)+I(t)\dot{\omega}(t), \\
& I(t)=R(t)I_0R(t)^T, \\
& \dot{I}(t)=\dot{R}(t)I_0R(t)^T+R(t)I_0\dot{R}(t)^T, \\
& \dot{R}(t)^T=[\omega(t)]R(t).
\end{split}
\end{equation}

The linear and angular velocities $v,\omega$ and accelerations $\dot{v},\dot{\omega}$ of a part can be calculated from its trajectory, and $R(t)$ is the rotation matrix of the part in frame $t$. The mass $M$ is set to $1$ since we do not set constraints on the attitude of forces on the fingers. We stack $\dot{P}$ and $\dot{L}$ into $\mathbf{b}$.

For each frame, we also calculate the force the fingers can apply on the object. First, we find all the contact points on the object mesh, which are less than 2mm from the fingers. To model frictional contact, we use four bases to approximate Coulomb's friction cone. We use 0.35 as the friction coefficient. We additionally add opposite force bases with the same coefficient variables on both parts of an articulated object, perpendicular to the spin axis of the object, modeling the articulation. We also add the supporting force basis of the part if the part is considered on the world's ground, which is to have an altitude above the lowest within 5mm.

Let $K$ denote the number of force bases. We compute the force and torque for each part in frame $t$:

\begin{equation}\label{eq:eval_force}
\begin{split}
& F(t)=\sum_{i=1}^K V_i(t)x_i(t)+Mg, \\
& \tau(t)=\sum_{i=1}^K[c_i(t)-o(t)]V_i(t)x_i(t),
\end{split}
\end{equation}

where $V$ is the force basis at each contact point, $c$ is the corresponding contact point, and $o$ is the part center of mass. $\mathbf{x}=[x_1(t), x_2(t), \cdots, x_K(t)]^T$ are the non-negative coefficients that we can apply along each force basis. Since both $F(t)$ and $\tau(t)$ in Equation~\eqref{eq:eval_force} are linear w.r.t. $\mathbf{x}$, we denote the right part of Equation~\eqref{eq:eval_force} as a linear transformation $\mathbf{A}\mathbf{x}+\mathbf{b}$, where $\mathbf{A} \in \mathbb{R}^{(3+3)\times K}$ and $\mathbf{b} \in \mathbb{R}^{3+3}$.

Given a pose trajectory for an object part, we can approximate the velocity and acceleration of the object part, hence computing the expected values of $F(t)$ and $\tau(t)$ that could force the object to move along such a trajectory. Let $\mathbf{c}$ denotes the 6D concatenation $[F(t), \tau(t)]^T$. We thus find an optimal $\mathbf{x}$ that minimize $\lVert\mathbf{A}\mathbf{x}+\mathbf{b}-\mathbf{c}\rVert_2$ with the constraint $\mathbf{x}\ge 0$. Only if $\min_{\mathbf{x}} \lVert\mathbf{A}\mathbf{x}+\mathbf{b}-\mathbf{c}\rVert_2 < 0.01$ do we consider a frame is consistent between contact and object movement. As one of our evaluation metrics, we compute the proportion of such consistent frames among all video frames.

\subsection{Articulation Consistency}
\label{subsec:A_C}

We evaluate whether the hand pose can control the object state in a human-like manner for an articulated object with a single revolute joint. The key insight is that, for each part of such an articulated object, the torque imposed by a human hand should be along the direction of the revolute joint. We consider all the contact points on the object surface that are less than $2$mm from the fingers. To simulate the forces on the object, we first add the gravity as well as the supporting force of the world's ground into our calculation similar to Section~\ref{subsec:CM_Consist}. We then suppose that a unified force is applied along the normal direction of each contact point, and compute the torque of each force w.r.t. the revolute joint of the articulated object. We normalize these torques with the inertia of the object.

Let $\vec{d}$ denote the direction of the object revolute joint. For each object part, we compute $E_{Art}=\max_{\tau} \tau \cdot \vec{d}$, where $\tau$ is the torque applied at a contact point. We consider a video frame achieves articulation consistency, only if each object part in this frame satisfies $E_{Art}>0.3$. We calculate the proportion of such qualified video frames as one of our evaluation metrics.

\subsection{Perceptual Score}
\label{subsection:P_S}

We collect human perceptual scores to judge the naturalness of the motion sequences.

We invite 23 people who are not familiar with motion synthesis and have no information on our method or any of the baselines to rate the generated animation videos from both our approach and baselines. These people are given 10 different result videos per method per object category, where all videos are shuffled, and the corresponding method names are blind to the people. After that, they are required to rate each video from 1 to 5. The scoring rules are:

\begin{itemize}
    \item 1 point: This video is very different from human behaviors, with lots of physical unrealities such as penetration and hand-object separation;
    \item 3 points: This video is human-like and physically plausible to some extent, but the tester can still detect the difference with human behavior or obvious physical defects;
    \item 5 points: This video is basically consistent with human behavior and is physically realistic.
\end{itemize}

For each method, we first compute the mean rating score of each object category and then report the average score among all categories in the main paper.

\section{Experimental Details}
\label{sec:experimental_details}

Given triangular part meshes $\{\mathbf{M}_i\}_{i=1}^N$ of a manipulated object, we sample 1000 points from each part mesh. We use a batch size of 64 for training, and the training procedure contains 500 epochs for Laptops and 1000 epochs for other categories. To balance the effects of different loss functions, we empirically set $\lambda_{flag}=0.1$, $\lambda_{pos}=500$, $\lambda_{dir}=100$, $\lambda_{tip}=100$, $\lambda_{vec}=1$, and $\lambda_{kld}=5$ during training.

In our synthesizer, we first optimize MANO hand pose parameter $\theta$ in 2000 epochs for fitting finger embedding. We simply set $\lambda_{\mathrm{tip}}=50$, $\lambda_{\mathrm{joint}}=1$, and $\lambda_{\mathrm{smooth}}=0.05$ and $1000$ respectively for the 45D MANO pose parameters and 3D wrist position parameters in $\theta$. To further optimize contact and penetration, we then iteratively use 6 steps to progressively improve the $\theta$, while in each step, the optimization process contains 500 epochs. We empirically set $\lambda_{\mathrm{contact}}=80$, $\lambda_{\mathrm{trans}}=1$, $\lambda_v=5$ and $\lambda_a=20$. To progressively improve the smoothness of our synthesis results, the parameter $\lambda_{\mathrm{smooth}}$ is set to $1$ in the first two steps, $10$ in the following two steps and $500$ in the last two steps.

\section{Data Processing for HOI4D}
\label{sec:data_processing}

To better leverage the HOI4D \cite{hoi4d} dataset for synthesis purposes, we performed several augmentation and modification steps to the raw data. We first split the object instances into training and testing sets in a proportion of $7:3$. Due to the limitation of the data collection method, the original HOI4D has a non-negligible problem of noise and penetration. To eliminate the noise, we extract several keyframes for each segment in training data and perform smooth interpolations between the keyframes. To solve the penetration problem, we use a contact optimization technique that is almost the same as our synthesizer module, in which we manually specify the contact points in each keyframe.

\section{Additional Baseline}
\label{sec:additional_baseline}

\begin{table*}[t]
\centering
\begin{tabular}{cccccccccc}
    \toprule[2pt]
    &\multicolumn{3}{c}{Pliers} & \multicolumn{3}{c}{Scissors}  & \multicolumn{3}{c}{Laptop}  \\ 
    & Pen $(\%)\downarrow$ & Mov $\uparrow$ & Art $\uparrow$ & Pen $(\%)\downarrow$ & Mov $\uparrow$ & Art $\uparrow$ & Pen $(\%)\downarrow$ & Mov $\uparrow$ & Art $\uparrow$  \\
    \midrule
    Ground Truth & 0.000 & 1.000 & 1.000 & 0.046 & 1.000 & 0.970 & 0.316 & 1.000 & 1.000 \\
    \midrule
    GraspTTA & 0.555 & 0.779 & 0.420 & 0.454 & 0.993 & 0.849 & 5.211 & \textbf{1.000} & 0.997 \\
    GraspTTA+TOCH & 0.124 & 0.918 & 0.511 & 0.124 & 0.947 & 0.298 & 1.596 & \textbf{1.000} & 0.978 \\
    CAMS (Ours) & \textbf{0.004} & \textbf{1.000} & \textbf{1.000} & \textbf{0.080} & \textbf{0.999} & \textbf{0.989} & \textbf{0.906} & \textbf{1.000} & \textbf{1.000} \\
    \midrule[2pt]
    & \multicolumn{3}{c}{Kettle}  &  \multicolumn{3}{c}{Overall} \\ 
    & Pen $(\%)\downarrow$ & Mov $\uparrow$ & Art $\uparrow$ & Pen $(\%)\downarrow$ & Mov $\uparrow$ & Art $\uparrow$  \\
    \midrule
    Ground Truth & 0.602 & 1.000 & N/A & 0.241 & 1.000 & 0.990 \\
    \midrule
    GraspTTA & 4.852 & 0.586 & N/A & 2.768 & 0.839 & 0.755 \\
    GraspTTA+TOCH & 2.002 & 0.897 & N/A & 0.961 & 0.941 & 0.596 \\
    CAMS (Ours) & \textbf{0.098} & \textbf{0.915} & N/A & \textbf{0.272} & \textbf{0.978} & \textbf{0.996} \\
    \bottomrule[2pt]
    
\end{tabular}
\caption{\textbf{Quantitative results compared with GraspTTA \cite{grasptta} and GraspTTA+TOCH \cite{TOCH}.} ``Pen'' denotes the average percentage of hand vertices penetrated in the object. ``Mov'' denotes the average proportion of frames that are contact-movement consistent. ``Art'' denotes the average proportion of frames that are articulation consistent.}
\vspace{-0.5cm}
\label{tab:supp_baseline_result}
\end{table*}

\textbf{GraspTTA\cite{grasptta}+TOCH\cite{TOCH}:} TOCH was developed to refine the hand poses given a coarse hand-object manipulation. Benefiting from the dense field representation, TOCH could precisely sense the local geometry of contact. Thus we additionally implement a baseline that further refines the result of GraspTTA using TOCH. To better adapt the imperfect generation results from ManipNet, we train TOCH networks with ground truth manipulation trajectories added with random noise, and test in unseen manipulation animations generated from GraspTTA.

\textbf{Quantitative result:}
As shown in Table~\ref{tab:supp_baseline_result}, GraspTTA+TOCH could generate physically more realistic results than simply using GraspTTA, whereas our approach still significantly outperforms the baselines.

\section{Additional Ablation Studies}
\label{sec:additional_ablation}

\begin{table}[t]
\centering
\begin{tabular}{cccc}
    \toprule[2pt]
    & Pen $(\%)\downarrow$ & Mov $\uparrow$ & Art $\uparrow$  \\
    \midrule
    Ground Truth & 0.000 & 1.000 & 1.000  \\
    \midrule
    CAMS (w/o Obj Can) & 0.147 & \textbf{1.000} & \textbf{1.000} \\
    CAMS (w/o Contact Can) & 0.021 & \textbf{1.000} & 0.879 \\
    CAMS (Abs Finger) & 0.009 & 0.998 & \textbf{1.000} \\
    CAMS & \textbf{0.004} & \textbf{1.000} & \textbf{1.000} \\
    \bottomrule[2pt]
    
\end{tabular}
\caption{\textbf{Additional ablation studies on the ``Pliers'' category.}}
\vspace{-0.5cm}
\label{tab:ablation_supp}
\end{table}

\textbf{Object-centric Canonicalization}
We ablate the root-level canonicalization and thus generate contact reference frames directly in the original object frame rather than the scale-normalized one. As shown in Table~\ref{tab:ablation_supp} (2nd line), our CAMS performs worse without object-centric canonicalization, and the generalizability of our framework also decreases.

\textbf{Contact-centric Canonicalization}
We also design experiments to demonstrate the necessity of canonicalizing finger embedding into the contact reference frames. Table~\ref{tab:ablation_supp} (3rd line) shows that both penetration rate and articulation rate significantly decrease after removing the contact-centric canonicalization, indicating that our contact-centric canonicalization could help improve the synthesis quality.

\textbf{Absolute Finger Embedding}
Instead of representing the canonicalized finger embedding as $\mathbf{F}_i=(\mathbf{J}^{tip}_i, \mathbf{D}^{dip}_i, \mathbf{D}^{pip}_i,\mathbf{D}^{mcp}_i,\mathbf{D}^{root}_i)$, we use similar representations to $\mathbf{J}^{tip}_i$ for other joints, denoted as $\mathbf{F}_i^{abs}=(\mathbf{J}^{tip}_i, \mathbf{J}^{dip}_i, \mathbf{J}^{pip}_i, \mathbf{J}^{mcp}_i, \mathbf{J}^{root}_i)$, which are absolute positions of the $i$-th finger's joints respectively. Table~\ref{tab:ablation_supp} (4th line) shows that using the absolute position for finger joints could harm the whole framework.
% And there is conflict in generated finger embeddings using absolute representations sometimes.

% \section{Visualization}
% \label{sec:visualization}

% Please watch our \textbf{video} for more visual synthesis results.
